# Supplementary material for: The Effect of Hole Ice on the Propagation and Detection of Light in IceCube
Source: arXiv:1904.08422 source file (2019-04-17)
Supplement: Supplementary file 1 [file appendix.tex]

% Appendix
